# Supplementary material for: GD^2-NeRF: Generative Detail Compensation via GAN and Diffusion for One-shot Generalizable Neural Radiance Fields
Source: arXiv:2401.00616 source file (2024-03-29)
Supplement: Supplementary file 1 [file Appendix_Ablation_Resolution.tex]

\begin{table}[t]
    \small
    \setlength\tabcolsep{7.2pt}
    \caption{\textbf{Influence of the resolution of the intermediate feature map $\textbf{I}_m$.} }
    \label{tab:ablation_resolution}
    
    \begin{tabular}{l|cccc}
    \rowcolor[gray]{.9}
    \hline
    Methods          & $\uparrow$ PSNR                & $\uparrow$ SSIM               & $\downarrow$ LPIPS      & $\downarrow$ FID \\ \hline \hline
    
    OPP (8\times8) & 22.31 & 0.884 & 0.151 & 105.06 \\
    OPP (16\times16) & \textbf{23.69}      & \textbf{0.910}     & \textbf{0.091} & \textbf{39.29} \\
    OPP (32\times32) & OOM  & OOM  &  OOM  & OOM  \\
    
    \hline
    \end{tabular}
 
\end{table}
