# Supplementary material for: GD^2-NeRF: Generative Detail Compensation via GAN and Diffusion for One-shot Generalizable Neural Radiance Fields
Source: arXiv:2401.00616 source file (2024-03-29)
Supplement: Supplementary file 2 [file Appendix_Ablation_Weight_Function.tex]

\begin{table}[t]
     \caption{\textbf{Influence of $\alpha$ on ShapeNet.} RVBA is relatively robust to the choice of $\alpha$ on ShapeNet. We use $\alpha=1$ for all the ShapeNet experiments by default. }
    \label{tab:ablation_weight_func}
    \resizebox{\linewidth}{!}{
    
        \begin{tabular}{l|cccc}
        \rowcolor[gray]{.9}
        \hline
        Methods          & $\uparrow$ PSNR                & $\uparrow$ SSIM               & $\downarrow$ LPIPS      & $\downarrow$ FID \\ \hline \hline

     OG-NeRF (DPS)   & {23.64}                         & {0.909}                    & 0.108             &  61.07   \\
        Generative (DPS)   &  23.16                        & 0.902                    & {0.085}             &  41.35   \\  \hline \hline
        
 RVBA (\alpha=\frac{1}{2})
   &           23.61              & 0.908                          &     \textbf{0.087}               &  \textbf{37.49}    \\
  
   RVBA (\alpha=1)         
    &  \textbf{23.69}                       &   \textbf{0.910}                        &      0.091              &  39.29    \\
    
    RVBA (\alpha=2)
    &    \textbf{23.69}                     &  \textbf{0.910}                         &      0.097              &  44.87    \\

         \hline
        \end{tabular}
    }
\end{table}
