# Supplementary material for: GD^2-NeRF: Generative Detail Compensation via GAN and Diffusion for One-shot Generalizable Neural Radiance Fields
Source: arXiv:2401.00616 source file (2024-03-29)
Supplement: Supplementary file 3 [file Appendix_Ablation_Weight_Function_DTU.tex]

\begin{table}[t]
     \caption{\textbf{Influence of $\alpha$ on DTU dataset.} The real-world dataset DTU is more complex than ShapeNet, which leads to the OG-NeRF paradigm becomes blurry faster than on ShapeNet. Therefore, $\alpha < 1$ is preferred. We use $\alpha=\frac{1}{5}$ by default considering it achieves a good balance between fidelity and sharpness. }
    \label{tab:ablation_weight_func_dtu}
    \resizebox{\linewidth}{!}{
    
        \begin{tabular}{l|cccc}
        \rowcolor[gray]{.9}
        \hline
        Methods          & $\uparrow$ PSNR                & $\uparrow$ SSIM               & $\downarrow$ LPIPS      & $\downarrow$ FID \\ \hline \hline

     OG-NeRF (DPS)   & {16.16}                         & {0.551}                    & 0.438             &  207.47   \\
        Generative (DPS)   &  16.06                        & 0.540                    & 0.372            &  149.99   \\  \hline \hline
        
    RVBA (\alpha=1)
    &          16.19             & 0.554                          &     0.429              & 187.15    \\
  
    RVBA (\alpha=\frac{1}{3})         
    &  \textbf{16.20}                       &   \textbf{0.555}                        &      0.392              &  150.07    \\
    
    RVBA (\alpha=\frac{1}{5})
    &    16.18	
                  &  0.552	                      &     0.381	            &  145.12  \\
    RVBA (\alpha=\frac{1}{7})
    &    16.16	
                  &  0.550	                      &     \textbf{0.377}	            &  \textbf{144.98}  \\
    % RVBA (\alpha=\frac{1}{9})
    % &    16.14	
    %               &  0.548	                      &     \textbf{0.375}	            &  146.25  \\
    \hline
    \end{tabular}
    }
\end{table}
