# Supplementary material for: GD^2-NeRF: Generative Detail Compensation via GAN and Diffusion for One-shot Generalizable Neural Radiance Fields
Source: arXiv:2401.00616 source file (2024-03-29)
Supplement: Supplementary file 4 [file Appendix_Ablation_Weight_Function_Learned.tex]

\begin{table}[t]
     \caption{\textbf{Comparisons between the learned weight masks and the manually designed weighting function.} ``\dag'' indicates a two-stage training is required. }
    \label{tab:ablation_weight_func_learned}
    \resizebox{\linewidth}{!}{
    
        \begin{tabular}{l|cccc}
        \rowcolor[gray]{.9}
        \hline
        Methods          & $\uparrow$ PSNR                & $\uparrow$ SSIM               & $\downarrow$ LPIPS      & $\downarrow$ FID \\ \hline \hline

     OG-NeRF (DPS)   & {23.64}                         & {0.909}                    & 0.108             &  61.07   \\
        Generative (DPS)   &  23.16                        & 0.902                    & {0.085}             &  41.35   \\  \hline \hline

    RVBA (Learned)\dag
    &    {23.59}                     &  {0.909}                         &      0.092              &  44.44    \\
    
    RVBA (Manual)         
    &  \textbf{23.69}                       &   \textbf{0.910}                        &      \textbf{0.091}              &  \textbf{39.29}    \\
         \hline
        \end{tabular}
    }
    \vspace{-2mm}
\end{table}
